# Supplementary material for: Multi-Agent Off-Policy TD Learning: Finite-Time Analysis with Near-Optimal Sample Complexity and Communication Complexity
Source: arXiv:2103.13147 source file (2021-03-24)
Supplement: Supplementary file 1 [file appendix.tex]

\clearpage
\onecolumn
\appendix
