# Supplementary material for: Multi-Agent Off-Policy TD Learning: Finite-Time Analysis with Near-Optimal Sample Complexity and Communication Complexity
Source: arXiv:2103.13147 source file (2021-03-24)
Supplement: Supplementary file 2 [file lemma_sync.tex]

\section{Proof of Theorem \ref{thm_sync}}

\thmconv*

\begin{proof}[Proof of Theorem \ref{thm_sync}]
	\begin{align}
		&\mathbb{E}\big[\|\overline{w}_{t+1}-w_t^*\|^2\big|\mathcal{F}_t\big]\nonumber\\
		&\le \mathbb{E}\big[\|\overline{w}_{t}+\beta(\overline{A}_{t}\overline{\theta}_{t}+\overline{\overline{b}}_{t}+\overline{C}_{t}\overline{w}_{t})-w_t^*\|^2 \big|\mathcal{F}_t\big] \nonumber\\
		&\le \|\overline{w}_{t}-w_t^*\|^2 + 2\beta(\overline{w}_{t}-w_t^*)^{\top}\mathbb{E}\big[\overline{A}_{t}\overline{\theta}_{t}+\overline{\overline{b}}_{t}+\overline{C}_{t}\overline{w}_{t}\big|\mathcal{F}_t\big] + \beta^2 \mathbb{E}\big[\big\|\overline{A}_{t}\overline{\theta}_{t}+\overline{\overline{b}}_{t}+\overline{C}_{t}\overline{w}_{t}\big\|^2\big|\mathcal{F}_t\big] \nonumber\\
		&\stackrel{(i)}{\le} \|\overline{w}_{t}-w_t^*\|^2 + \beta\Big(\frac{2c_{\text{sd}}}{T}-\lambda_{2}\Big) \big\|\overline{w}_{t}-w_t^*\big\|^2 + \frac{3\beta c_{\text{var,2}}\Omega_{A}^2}{T\lambda_{2}} \big\|\overline{\theta}_{t}-\theta^*\big\|^2 + \frac{3\beta c_{\text{var,2}}}{T\lambda_{2}} \big(\Omega_{A}^2\big\|\theta^*\big\|^2 + \Omega_{b}^2\big) \nonumber\\
		&\quad +\frac{4\beta^2 c_{\text{var,2}}\Omega_{A}^2}{T} \|\overline{\theta}_t-\theta^*\|^2 + 4\beta^2 \big\|\overline{w}_{t}-w_t^*\big\|^2  + \frac{4\beta^2 c_{\text{var,2}}}{T} (\Omega_{A}^2\|\theta^*\|^2 + \Omega_{b}^2) \nonumber\\
		&\le \Big[1+\beta\Big(\frac{2c_{\text{sd}}}{T}-\lambda_{2}+4\beta\Big)\Big] \|\overline{w}_{t}-w_t^*\|^2 + \frac{\beta c_{\text{var,2}}\Omega_{A}^2}{T} \Big(\frac{3}{\lambda_{2}}+4\beta\Big) \big\|\overline{\theta}_{t}-\theta^*\big\|^2 + \frac{\beta c_{\text{var,2}}}{T} \Big(\frac{3}{\lambda_{2}}+4\beta\Big) \big(\Omega_{A}^2\big\|\theta^*\big\|^2 + \Omega_{b}^2\big) \nonumber\\
		&\stackrel{(ii)}{\le} \Big(1-\frac{\beta\lambda_{2}}{2}\Big) \|\overline{w}_{t}-w_t^*\|^2 + \frac{7\beta c_{\text{var,2}}\Omega_{A}^2}{T\lambda_{2}} \big\|\overline{\theta}_{t}-\theta^*\big\|^2 + \frac{7\beta c_{\text{var,2}}}{T\lambda_{2}} \big(\Omega_{A}^2\big\|\theta^*\big\|^2 + \Omega_{b}^2\big) \label{wdelay_err}
	\end{align}
	where (i) uses eqs. \eqref{SGbias_w} \& \eqref{SGvar_w}, and (ii) uses the conditions that $\frac{4c_{\text{sd}}}{T}+8\beta\le\lambda_{2}$ and $\beta\le\frac{1}{\lambda_{2}}$. Hence,
	\begin{align}
	&\mathbb{E}\big[\|\overline{w}_{t+1}-w_{t+1}^*\|^2\big|\mathcal{F}_t\big]\nonumber\\
	&\stackrel{(i)}{\le} \Big(1+\frac{1}{2[2/(\beta\lambda_{2})-1]}\Big) \mathbb{E}\big[\|\overline{w}_{t+1}-w_t^*\|^2\big|\mathcal{F}_t\big] + \big[1+2\big(2/(\beta\lambda_{2})-1\big)\big] \mathbb{E}\big[\|w_{t+1}^*-w_t^*\|^2\big|\mathcal{F}_t\big] \nonumber\\
	&\stackrel{(ii)}{\le} \frac{4/(\beta\lambda_{2})-1}{2[2/(\beta\lambda_{2})-1]} \Big[\Big(1-\frac{\beta\lambda_{2}}{2}\Big) \|\overline{w}_{t}-w_t^*\|^2 + \frac{7\beta c_{\text{var,2}}\Omega_{A}^2}{T\lambda_{2}} \big\|\overline{\theta}_{t}-\theta^*\big\|^2 + \frac{7\beta c_{\text{var,2}}}{T\lambda_{2}} \big(\Omega_{A}^2\big\|\theta^*\big\|^2 + \Omega_{b}^2\big) \Big]\nonumber\\ 
	&\quad+\Big(\frac{4}{\beta\lambda_2}-1\Big) \mathbb{E}\big[\|C^{-1}A(\overline{\theta}_{t+1}-\overline{\theta}_{t})\|^2\big|\mathcal{F}_t\big] \nonumber\\
	&\stackrel{(iii)}{\le} \Big(1-\frac{\beta\lambda_{2}}{4}\Big)\|\overline{w}_{t}-w_t^*\|^2 + \frac{14\beta c_{\text{var,2}}\Omega_{A}^2}{T\lambda_{2}} \big\|\overline{\theta}_{t}-\theta^*\big\|^2 + \frac{14\beta c_{\text{var,2}}}{T\lambda_{2}} \big(\Omega_{A}^2\big\|\theta^*\big\|^2 + \Omega_{b}^2\big) \nonumber\\
	&\quad +\Omega_{A}^2\|C^{-1}\|^2 \Big(\frac{4}{\beta\lambda_2}-1\Big) \mathbb{E}\big[ \big\|\alpha\big(\overline{A}_t\overline{\theta}_t+\overline{\overline{b}}_t+\overline{B}_t\overline{w}_t\big)\big\|^2 \big|\mathcal{F}_t\big] \nonumber\\
	&\stackrel{(iv)}{=} \Big(1-\frac{\beta\lambda_{2}}{4}\Big)\|\overline{w}_{t}-w_t^*\|^2 + \frac{14\beta c_{\text{var,2}}\Omega_{A}^2}{T\lambda_{2}} \big\|\overline{\theta}_{t}-\theta^*\big\|^2 + \frac{14\beta c_{\text{var,2}}}{T\lambda_{2}} \big(\Omega_{A}^2\big\|\theta^*\big\|^2 + \Omega_{b}^2\big) \nonumber\\
	&\quad +\frac{4\alpha^2}{\beta\lambda_2}\Omega_{A}^2\|C^{-1}\|^2 \Big[10\Omega_{A}^2\big(1+\Omega_{B}^2\|C^{-1}\|^2\big)\big\|\overline{\theta}_{t}-\theta^*\big\|^2 + 5\Omega_{B}^2\big\|\overline{w}_{t}-w_t^*\big\|^2 \nonumber\\
	&\quad +\frac{5}{T} 
	\big[c_{\text{var,3}}\Omega_{A}^2\big\|\theta^*\big\|^2+c_{\text{var}}\Omega_{b}^2\big(1+\Omega_{B}^2\|C^{-1}\|^2\big)\big] \Big] \nonumber\\
	&\stackrel{(v)}{=} \Big(1-\frac{\beta\lambda_{2}}{4}+\frac{\alpha^2 c_1}{\beta}\Big)\|\overline{w}_{t}-w_t^*\|^2 + \Big(\frac{\beta c_2}{T} + \frac{\alpha^2 c_3}{\beta}\Big) \big\|\overline{\theta}_{t}-\theta^*\big\|^2 + \Big(\frac{\beta c_4}{T} + \frac{\alpha^2 c_5}{T\beta}\Big) \nonumber\\
	&\stackrel{(vi)}{\le} \Big(1-\frac{\beta\lambda_{2}}{8}\Big)\|\overline{w}_{t}-w_t^*\|^2 + \Big(\frac{\beta c_2}{T} + \frac{\alpha^2 c_3}{\beta}\Big) \big\|\overline{\theta}_{t}-\theta^*\big\|^2 + \frac{2\beta c_4}{T} \label{w_err_iter}
	\end{align}
	where (i) uses the inequality that $\|a+b\|^2\le (1+\gamma)\|a\|^2+(1+\gamma^{-1})\|b\|^2$ for any $a,b\in\mathbb{R}^d$ and $\gamma>0$, (ii) uses eq. \eqref{wdelay_err}, (iii) uses $\beta\le\frac{1}{\lambda_{2}}$ (this implies that $\frac{4/(\beta\lambda_{2})-1}{2[2/(\beta\lambda_{2})-1]}\le\frac{3}{2}<2$) and eqs. \eqref{theta_iter_avg1} \& \eqref{bound_A}, (iv) uses eq. \eqref{SGvar_theta}, (v) denotes that $c_1=\frac{20}{\lambda_2}\Omega_{A}^2\Omega_{B}^2\|C^{-1}\|^2$, $c_2=\frac{14 c_{\text{var,2}}\Omega_{A}^2}{\lambda_{2}}$, $c_3= \frac{40}{\lambda_2}\Omega_{A}^4\|C^{-1}\|^2 \big(1+\Omega_{B}^2\|C^{-1}\|^2\big)$, $c_4=\frac{14 c_{\text{var,2}}}{\lambda_{2}} \big(\Omega_{A}^2\big\|\theta^*\big\|^2 + \Omega_{b}^2\big)$, $c_5=\frac{20}{\lambda_2}\Omega_{A}^2\|C^{-1}\|^2 \big[c_{\text{var,3}}\Omega_{A}^2\big\|\theta^*\big\|^2+c_{\text{var}}\Omega_{b}^2\big(1+\Omega_{B}^2\|C^{-1}\|^2\big)\big]$, (vi) uses the conditions that $\alpha\le \beta \min\Big(\frac{1}{3}\sqrt{\frac{\lambda_2}{c_1}},  \sqrt{\frac{c_4}{c_5}}\Big)$. 
	
	\begin{align}
	&\mathbb{E}\big[\|\overline{\theta}_{t+1}-\theta^*\|^2\big|\mathcal{F}_t\big]\nonumber\\
	&\le \mathbb{E}\big[\|\overline{\theta}_{t}+\alpha\big(\overline{A}_{t}\overline{\theta}_{t}+\overline{\overline{b}}_{t}+\overline{B}_{t}\overline{w}_{t}\big)-\theta^*\|^2 \big|\mathcal{F}_t\big] \nonumber\\
	&\le \|\overline{\theta}_{t}-\theta^*\|^2 + 2\alpha\big(\overline{\theta}_{t}-\theta^*\big)^{\top}\mathbb{E}\big[\overline{A}_{t}\overline{\theta}_{t}+\overline{\overline{b}}_{t}+\overline{B}_{t}\overline{w}_{t}\big|\mathcal{F}_t\big] + \alpha^2 \mathbb{E}\big[\big\|\overline{A}_{t}\overline{\theta}_{t}+\overline{\overline{b}}_{t}+\overline{B}_{t}\overline{w}_{t}\big\|^2\big|\mathcal{F}_t\big] \nonumber\\
	&\stackrel{(i)}{\le} \Big[1+\alpha\Big( \frac{2c_{\text{var,3}}\Omega_{A}^2}{T\lambda_{1}}-\lambda_{1} \Big)+10\alpha^2\Omega_{A}^2\big(1+\Omega_{B}^2\|C^{-1}\|^2\big)\Big]\|\overline{\theta}_{t}-\theta^*\|^2 +\alpha\Omega_{B}^2 \Big(\frac{4}{\lambda_{1}}+5\alpha\Big)\big\|\overline{w}_{t}-w_t^*\big\|^2 \nonumber\\ 
	&\quad + \frac{\alpha}{T} \Big(\frac{4}{\lambda_{1}}+5\alpha\Big)
	\big[c_{\text{var,3}}\Omega_{A}^2\big\|\theta^*\big\|^2+c_{\text{var}}\Omega_{b}^2\big(1+\Omega_{B}^2\|C^{-1}\|^2\big)\big] \nonumber\\
	&\stackrel{(ii)}{\le} \Big(1-\frac{\alpha\lambda_{1}}{2}\Big)\|\overline{\theta}_{t}-\theta^*\|^2 + \frac{9\alpha\Omega_{B}^2}{\lambda_{1}} \big\|\overline{w}_{t}-w_t^*\big\|^2 + \frac{9\alpha}{T\lambda_{1}} \big[c_{\text{var,3}}\Omega_{A}^2\big\|\theta^*\big\|^2+c_{\text{var}}\Omega_{b}^2\big(1+\Omega_{B}^2\|C^{-1}\|^2\big)\big] \nonumber\\
	&\stackrel{(iii)}{\le} \Big(1-\frac{\alpha\lambda_{1}}{2}\Big)\|\overline{\theta}_{t}-\theta^*\|^2 + \alpha c_6 \big\|\overline{w}_{t}-w_t^*\big\|^2 + \frac{\alpha c_7}{T} \label{theta_err_iter}
	\end{align}
	where (i) uses eqs. \eqref{SGbias_theta} \& \eqref{SGvar_theta}, (ii) uses the conditions that $T\ge \frac{8c_{\text{var,3}}\Omega_{A}^2}{\lambda_{1}^2}$ and that $\alpha\le \min\Big[\frac{\lambda_1}{40\alpha\Omega_{A}^2\big(1+\Omega_{B}^2\|C^{-1}\|^2\big)},\frac{1}{\lambda_{1}}\Big]$, and (iii) uses the notations that $c_6=\frac{9\Omega_{B}^2}{\lambda_{1}}$ and that $c_7=\frac{9}{\lambda_{1}}  \big[c_{\text{var,3}}\Omega_{A}^2\big\|\theta^*\big\|^2+c_{\text{var}}\Omega_{b}^2\big(1+\Omega_{B}^2\|C^{-1}\|^2\big)\big]$.
	
	Taking expectation on both sides of eqs. \eqref{w_err_iter}\&\eqref{theta_err_iter} and summing up the two inequalities yield that 
	\begin{align}
		&{\mathbb{E}(\|\overline{\theta}_{t+1}-\theta^*\|^2)} + {\mathbb{E}(\|\overline{w}_{t+1}-w_{t+1}^*\|^2)} \nonumber\\
		&\le \Big(1-\frac{\alpha\lambda_{1}}{2}+\frac{\beta c_2}{T} + \frac{\alpha^2 c_3}{\beta}\Big) \mathbb{E}(\|\overline{\theta}_{t}-\theta^*\|^2) + \Big(1-\frac{\beta\lambda_{2}}{8}+\alpha c_6\Big) \mathbb{E}(\|\overline{w}_{t}-w_{t}^*\|^2) + \frac{\alpha c_7+2\beta c_4}{T} \nonumber\\
		&\stackrel{(i)}{\le} \Big(1-\frac{\alpha\lambda_{1}}{4}\Big) \mathbb{E}(\|\overline{\theta}_{t}-\theta^*\|^2) + \Big(1-\frac{\beta\lambda_{2}}{16}\Big) \mathbb{E}(\|\overline{w}_{t}-w_{t}^*\|^2) + \frac{3\beta c_4}{T} \nonumber\\
		&\stackrel{(ii)}{\le} \Big(1-\frac{\alpha\lambda_{1}}{4}\Big) \big[\mathbb{E}(\|\overline{\theta}_{t}-\theta^*\|^2)+\mathbb{E}(\|\overline{w}_{t}-w_{t}^*\|^2)\big] + \frac{3\beta c_4}{T} \nonumber
	\end{align}
	where (i) uses the conditions that $T\ge \frac{8\beta c_2}{\alpha \lambda_1}$ and that $\alpha\le\beta \min \Big(\frac{c_6\lambda_2}{16}, \frac{\lambda_1}{8c_3}, \frac{c_4}{c_7}\Big)$, and (ii) uses the condition that $\alpha\le \frac{\beta\lambda_2}{4\lambda_1}$. Iterating the inequality above proves eq. \eqref{sum_err}
\end{proof}

%\thmconv*
%
%\begin{proof}[Proof of Theorem \ref{thm_sync}]
%
%	\begin{align}
%		\mathbb{E}\big(\|\theta_{m,T'}-\theta^*\|^2\big)&\le 2\mathbb{E}\big(\|\theta_{m,T'}-\overline{\theta}_{T'}\|^2\big)+2\mathbb{E}\big(\|\overline{\theta}_{T'}-\theta_{T'}^*\|^2\big)\nonumber\\
%		&\le 2\mathbb{E}\big(\big\|\Delta \Theta_{T'}\big\|_F^2\big)+2\mathbb{E}\big(\|\overline{\theta}_{T'}-\theta_{T'}^*\|^2\big)\nonumber\\
%		&\stackrel{(i)}{\le} 2\Big(\frac{1+\sigma_2^V}{2}\Big)^{T'} \big[\big\|\Delta \Theta(0)\big\|_F + \big\|\Delta W(0)\big\|_F\big] + 2\Big(1-\frac{\alpha\lambda_{1}}{4}\Big)^{T'} \big[\|\overline{\theta}_{0}-\theta^*\|^2+\|\overline{w}_{0}-w_{0}^*\|^2\big]\nonumber\\
%		&\quad +(\alpha+\beta)\frac{4\sqrt{M}\Omega_{b}}{1-\sigma_2^V} + \frac{24\beta c_4}{\alpha T\lambda_1}, \nonumber
%	\end{align}
%	where (i) uses eqs. \eqref{consensus1}\&\eqref{sum_err} (Notice that the conditions in Theorem \ref{thm_sync} cover those in Lemmas \ref{lemma_consensus1} \& \ref{lemma_avgrate1}, so the two Lemmas hold.). Therefore, when $\alpha,\beta=\mathcal{O}(\epsilon)$, $T=\mathcal{O}(\epsilon^{-1})$, $T'=\mathcal{O}\big[\epsilon^{-1}\ln(\epsilon^{-1})\big]$, we have $\mathbb{E}\big(\|\theta_{m,T'}-\theta^*\|^2\big)\le \mathcal{O}(\epsilon)$. 
%\end{proof}
